# Supplementary material for: A Unified View of Label Shift Estimation
Source: arXiv:2003.07554 source file (2020-10-16)
Supplement: Supplementary file 1 [file appendix.tex]

\onecolumn

% \section{Proofs from section~\ref{subsec:unified}} \label{sec:Appendixbgr}
% \begin{prop}\label{prop:calibA}
% Confusion matrix using the hard predictor in principle gives a per-label calibrated classifier on the source data. 
% \end{prop}

\section{Proofs from section~\ref{sec:unify}} \label{sec:AppendixA}

\begin{proof}[Proof of Proposition~\ref{prop:ltt-calib}]
\todoy{move proof to appendix}
We need to show $p_s(y|\f(\x)=c) = c$ for any $c$, which is $p_s(y|p_s(y|g(\x)) = c) = c$. \todoy{rigorously proving this is quite complicated as we need apply measure-theoretical definition of conditional probabilities.}
Let $\f^{-1}(c) = \{x:p_s(y|g(\x)) = c\}$. We have 
\[
\f^{-1}(c) = \cup_{\z:p_s(y|g(\x)=\z) = c} g^{-1}(\z) \,.
\]
Then we have
\begin{align*}
& p_s(\x \in \f^{-1}(c), y) \\
& = \sum_{\z:p_s(y|g(\x)=\z) = c} p_s(\x \in g^{-1}(\z), y) \\
& = \sum_{\z:p_s(y|g(\x)=\z) = c} p_s(\x \in g^{-1}(\z)) p_s(y|g(\x)=\z) \\
& = c \cdot \sum_{\z:p_s(y|g(\x)=\z) = c} p_s(\x \in g^{-1}(\z)) \\
& = c \cdot p_s(\x \in \f^{-1}(c)) \,.
\end{align*}
By definition of conditional distribution we can conclude that $p_s(y|\f(\x)=c) = c$.
\footnote{Our proof applies $p(a|b)=p(a, b)/p(b)$ where $p(b)$ is implicitly assumed to be positive. Writing the proof in measure theory will cover the general cases.}
\end{proof}

Restating the example from section~\ref{subsec:MLLS}.  
% in more general case with a probabilistic classifier. 
% \begin{example}\label{ex:necessary}
% Consider a mixture of two Gaussian with \allowdisplaybreaks{$\ps(x|y=1) \defeq \N(1, 1)$ and $\ps(x|y=-1) \defeq \N(-1, 1)$}. Let source mixing coefficients be $\frac{1}{2}$ each and target mixing coefficients be $\alpha, 1-\alpha$. With the thresholded classifier of the form $f(x) = [ \frac{1+\sign(x)}{2}, \frac{1-\sign(x)}{2}]$, the estimation error is $4\abs{\pt(x\ge0) - \alpha} = 4\times 0.1587\abs{1 - 2\alpha}$ which is non-zero for all $\alpha \ne \frac{1}{2}$ 
% \end{example}

\begin{example}
Consider a mixture of two Gaussians with \allowdisplaybreaks{$\ps(x|y=0) \defeq \N(\mu, 1)$ and $\ps(x|y=1) \defeq \N(-\mu, 1)$}. Assume source mixing coefficients be $\frac{1}{2}$ each and target mixing coefficients be $\alpha (\ne \frac{1}{2}), 1-\alpha $. Assume a class of probabilistic classifiers with threshold at $x=0$ that can be represented as $f(x) = [ \frac{1+(2c-1)\sign(x)}{2}, \frac{1-(2c-1)\sign(x)}{2}]$ with $c \in [0,1]$.  For such classifiers, the estimation error of population MLLS is given by $4\abs{\frac{\pt(x\le0) - c}{1-2c} - \alpha} = 4\abs{\frac{(1-2\alpha)(\ps(x\ge0|y=0) - c)}{1-2c}}$ which is zero for only if $c = \ps(x\ge0|y=0)$ for a non-degenerate classifier. 
\end{example}

\begin{proof}
The classifier $f(x)$ predicts class $0$ with probability $c$ and class $1$ with probability $1-c$ for $x\ge0$, and vice-versa for $x<0$. 
Using such a classifier, the weight estimator is given by, 
\begin{align*}    
 \widehat w &= \argmin_w \E{ \log\inner{f(x)}{w}}  \\
&\stackrel{\text{(i)}}{=} \argmin_{w_0} \left[ \int_{-\infty}^{0} \log((1-c)w_0 + c(2-w_0)) \pt(x) dx + \int_{0}^{\infty} \log(cw_0 + (1-c)(2-w_0)) \pt(x) dx \right]\\
&\stackrel{\text{(ii)}}{=} \argmin_{w_0} \left[  \log((1-c)w_0 + c(2-w_0)) \pt(x\le 0)  + \log(cw_0 + (1-c)(2-w_0)) \pt(x\ge 0) \right]
\end{align*}
where equality (i) follows from $w_1 = 2-w_0$ and the predictor function. (ii) follows from the fact that within each integral the  term inside log is independent of $x$.  
Differentiating wrt to $w_0$ we have: 
$$ \frac{1-2c}{2c + w_0 - 2cw_0} \pt(x\le 0) + \frac{2c-1}{2cw_0 + 2 -2c -w_0}\pt(x\ge 0) = 0  $$
$$ \frac{1}{2c + w_0 - 2cw_0} \pt(x\le 0) + \frac{-1}{2cw_0 + 2 -2c -w_0}(1 - \pt(x\le 0)) = 0  $$
$$ (2cw_0 + 2 -2c -w_0) \pt(x\le 0) - (2c + w_0 - 2cw_0)(1 - \pt(x\le 0)) = 0 $$
$$ 2\pt(x\le 0) - 2c - w_0 +2cw_0 = 0 $$
which gives $w_0 = \frac{2\pt(x\le 0) - 2c}{1-2c}$. Thus for population MLLS estimate, the estimation error is given by 
$$ || \widehat w - w^* ||_2 = 2 |w_0 - 2\alpha| = 4\abs{\frac{(1-2\alpha)(\ps(x\ge0|y=0) - c)}{1-2c}} $$
\end{proof}

\section{Proofs from section ~\ref{sec:finite}} \label{sec:AppendixB}
\begin{prop}  \label{prop:sc}
The optimization problem~\eqref{eq:mlls-sample} is self concordant.  
\end{prop}
\begin{proof}
By the property of self-concordance in $\Real^k$, $\LL_m(\w,\f)$ is self concordant if the function $\LL_m(\w + t\vv,\f)$ is self concordant for all $\w,\vv \in \inpt$. Clearly, $$\abs{ \LL^{\prime\prime\prime}_m(\w + t\vv,\f)} = 2\frac{\inner{\f}{\vv}^3}{\inner{\f}{\w + t\vv}^3} = 2\Big[\frac{\inner{\f}{\vv}^2}{\inner{\f}{\w + t\vv}^2}\Big]^{\frac{3}{2}} = 2\abs{\LL^{\prime\prime}_m(\w + t\vv,\f)}^{\frac{3}{2}}$$    
\end{proof}

\begin{prop} 
With the identifiability of the log-likelihood, the optimization problem~\eqref{eq:mlls-sample} is strongly convex.  
\end{prop}
\begin{proof} 
We absorb the negative sign in $\LL_m$ by reinterpreting it as negative log-likelihood. 

The Hessian matrix is given by
\[
\nabla_w^2\LL_m (\w, \f) = \frac{1}{m}\sum_{i=1}^m \nabla_w \mathcal{L}_1 (\x_i,\w, \f)^T \nabla_w  \mathcal{L}_1(\x_i, \w, \f)
\]
where $
\nabla \mathcal{L}_1 (\x_i, \w, \f) =  \begin{bmatrix} 
    \frac{f_1(x_i)}{\inner{\f(\x_i)}{\w}} 
    \dots  
    \frac{f_l(x_i)}{\inner{\f(\x_i)}{\w}} 
    \dots 
    \frac{ f_{k}(x_i) }{\inner{\f(\x_i)}{\w}} 
    \end{bmatrix}_{(k)}
$. 

By identifiability condition, we know that $\f$ is full row-rank. Let's assume that the Hessian is not positive definite i.e. there exist a non-zero vector $v \in \Real^{k-1}$ s.t. $\inner{\nabla \LL_1(\x_i, w, \f)}{v}=0$ for all $i=\{1\ldots m\}$. 
% By simple matrix multiplication we re-write 
% \begin{align*}    
% \begin{bmatrix} 
%     f_1(x_1) - f_k(x_1) \frac{\ps(y=1)}{\ps(y=k)} & \cdots &  f_1(x_m) - f_k(x_m) \frac{\ps(y=1)}{\ps(y=k)} \\
%     \vdots & \ddots & \vdots  \\
%     f_1(x_l) - f_k(x_1) \frac{\ps(y=l)}{\ps(y=k)} & \cdots &  f_l(x_m) - f_k(x_m) \frac{\ps(y=l)}{\ps(y=k)} \\
%     \vdots & \ddots & \vdots  \\
%     f_1(x_{k-1}) - f_k(x_1) \frac{\ps(y=k-1)}{\ps(y=k)} & \cdots &  f_{k-1}(x_m) - f_k(x_m) \frac{\ps(y=k-1)}{\ps(y=k)} \\
% \end{bmatrix}_{(k-1)\times m} &= \phantom{aaaaaaaaa}  \\  
% \begin{bmatrix} 
%     1 & 0 & 0 & \cdots & 0 & -\frac{p(y=1)}{p(y=k)} \\
%     0 & 1 & 0 & \cdots & 0 & -\frac{p(y=2)}{p(y=k)} \\
%     \vdots & \vdots & \vdots & \ddots &\vdots & \vdots \\
%     0 & 0 & 0 & \cdots & 1 & -\frac{p(y=k-1)}{p(y=k)} \\ 
% \end{bmatrix}_{(k-1)\times k}
% &\begin{bmatrix} 
%  f_1(x_1) & \cdots & f_1(x_n) \\
%  f_2(x_1) & \cdots & f_2(x_n) \\
%  \vdots & \ddots & \vdots \\
%  f_k(x_1) & \cdots & f_k(x_n) \\
% \end{bmatrix}_{k\times m}
% \end{align*}

% which shows that if $\f$ is span $\Real^k$ then for all $i=\{1\ldots m\}$ $\LL_1(\x_i, w, \f)$ span $\Real^{k-1}$. 
 
Consider $v$ as some linear combination of vectors in dimensions $k$ i.e. $v = \sum_{i=1}^{n} \alpha_i \nabla \LL_1(\x_i, w, \f)$ which implies $v^Tv = \sum_{i=1}^{n} \alpha_i \inner {\nabla \LL_1(\x_i, w, \f)}{v} =0$ giving contradiction on the assumption on non positive definiteness of Hessain. Hence, the Hessain matrix of the log-likelihood is positive definite.
\end{proof}

\begin{lemma} [\cite{tropp2015introduction} Matrix Chernoff Theorem 5.1.1] \label{lemma:troop}
Let $X_1, X_2, \ldots, X_n$ be a finite sequence of identically distributed independent, random, symmetric matrices with common dimention $k$. Assume $0 \preceq X \preceq R.I$ and $\mu_{\min}.I \preceq \E{X} \preceq \mu_{\max}.I$. With probability atleast $1-\delta$, 
\[ \lambda_{\min} = \text{min-eig}(\frac{1}{n}\sum_{i=1}^n X_i) \ge  \mu_{\min} - \sqrt{\frac{2R\mu_{\min}\log(\frac{k}{\delta})}{n}} 
\]
\end{lemma}
\begin{lemma}\label{lemma:err1}
Assume the identifiability condition of lemma~\ref{lemma:identi-1} hold true and the predictor function  $\fc$ is bounded below at the non zero entries of $\w^*$ i.e. for all $\x$ such that $\pt(\x)>0$, we have $\sum_{y=1}^k \fc_y(\x) \w^*_y \ge \tau$ for some universal constant $\tau$. Let $\smin^{\fc}$ be the minimum eigenvalue of the Fisher information.  With probability at least $1-\delta$ we have,  
$$||\wc - \w^*|| \defeq \comp \left(\frac{1}{\smin^{\fc}}\sqrt{\frac{\log(\frac{4}{\delta})}{m}}\right)$$
\end{lemma}

\begin{proof}
% Using identifiability, we have strong convexity on the empirical negative log-likelihood function which we represent with $\LL_m$ by absorbing the negative sign for simplified notation here on.
We represent empirical negative log-likelihood function with $\LL_m$ by absorbing the negative sign for simplified notation. Using Taylor expansion we have, 
$$ \LL_m(\wc, \fc) = \LL_m(\w^*, \fc) + \inner{\nabla \LL_m(\w^*, \fc)}{\wc - \w^*} + \frac{1}{2} (\wc - \w^*)^T \nabla^2\LL_m (\tilde\w, \fc)(\wc - \w^*) $$
where $\tilde\w \in [\wc, \w^*] $. With the assumption $<\fc, \w^*> \ge \tau$, we have $\nabla^2\LL_m (\tilde\w, \fc) \ge \frac{\tau^2}{\min \ps(y)^2} \nabla^2\LL_m (\w^*, \fc)$ \footnote{Instead we could have also used definition of self-concordance to get a lower bound with $\nabla^2\LL_m (\w^*, \fc)$.}.  Let $\kappa = \frac{\tau^2}{\min \ps(y)^2}$. Using this we get,  
$$ \LL_m(\wc, \fc) \ge \LL_m(\w^*, \fc) + \inner{\nabla \LL_m(\w^*, \fc)}{\wc - \w^*} + \frac{\kappa}{2} (\wc - \w^*)^T \nabla^2\LL_m (\w^*, \fc)(\wc - \w^*) $$
$$ \underbrace{\LL_m(\wc, \fc) - \LL_m(\w^*, \fc)}_{\RN{1}} - \inner{\nabla \LL_m(\w^*, \fc)}{\wc - \w^*}  \ge \frac{\kappa}{2} (\wc - \w^*)^T \nabla^2\LL_m (\w^*, \fc)(\wc - \w^*) $$
where term-$\RN{1}$ is less than zero as $\wc$ is the minimizer of empirical NLL $\LL_m(\w, \fc)$.
% $\mu^2\ge \smin({\nabla^2_w \LL_m (\w, \fc)})$ for $\w \in [\wc, \w^*]$. 
% We assume that $\mu$ is bounded above otherwise we trivially have strong guarantees on the $||\wc - w^*||$. 
% \todos[inline]{Improve this using tail bound on sigma min} 
Ignoring term-$\RN{1}$ and re-arranging a few terms we get:  
$$ - \inner{\nabla \LL_m(\w^*, \fc)}{\wc - \w^*}  \ge \frac{\kappa}{2} (\wc - \w^*)^T \nabla^2\LL_m (\w^*, \fc)(\wc - \w^*) $$
With first order optimality on $w^*$, $\inner{\nabla \LL(\w^*, \fc)}{\wc - \w^*} \ge 0$. Plugining in this, we have, 
$$ \inner{\nabla \LL(\w^*, \fc) - \nabla \LL_m(\w^*, \fc)}{\wc - \w^*}  \ge \frac{\kappa}{2} (\wc - \w^*)^T \nabla^2\LL_m (\w^*, \fc)(\wc - \w^*) $$
Using Holder's inequality on the LHS we have, 
$$  ||\nabla \LL(\w^*, \fc) - \nabla \LL_m(\w^*, \fc)||_2||\wc - \w^*||_2  \ge \frac{\kappa}{2} (\wc - \w^*)^T \nabla^2\LL_m (\w^*, \fc)(\wc - \w^*)$$
Let $\widehat \sigma_{\min}$ be the minimum eigenvalue of $\nabla^2\LL_m (\w^*, \fc)$. Using the fact that $(\wc - \w^*)^T \nabla^2\LL_m (\w^*, \fc)(\wc - \w^*) \ge \widehat \sigma_{\min} ||\wc - \w^* ||_2^2$, we get,     
\begin{equation} \label{eq:ineq1}
||\nabla \LL(\w^*, \fc) - \nabla \LL_m(\w^*, \fc)||_2  \ge \frac{\kappa \widehat \sigma_{\min}}{2} ||\wc - \w^* ||_2   
\end{equation}

% Consider $\E{\nabla \LL_m(\w^*, \fc)}$ $=  \E{\sum_{i=1}^m \frac{\nabla \LL_1 (\x_i, \w^*, \fc)}{m}} $ $= \E{\nabla \LL_1 (\x, \w^*, \fc)}$. 
% Consider one single entry in the vector, $$  \E{\nabla \LL_1 (\x, \w^*, \fc)}_l =  \int_{\x} \frac{f^c_l(\x) - f^c_k(\x) \frac{\ps(y=l)}{\ps(y=k)} }{\inner{\fc(\x)}{\w^*}} \pt(\x) d\x $$ 
% $$= \int_{\x} \frac{\Big(  \ps^c(y=l|\x) - \ps^c(y=k|\x) \frac{\ps(y=l)}{\ps(y=k)} \Big) \ps(x)}{\sum_{y=1}^k \ps^c(y|\x_i)w^*_j \ps(\x)}  \pt(\x) d\x$$ \todos{Change this after the proof of consistency to include indicators.}
% $$ = \int_{\x} \Big(  \ps^c(y=l|x_i) -  \ps^c(y=k|x_i) \frac{\ps(y=l)}{\ps(y=k)} \Big) \ps(\x) d\x  = 0$$ 

% With the bounded assumption on $\frac{\nabla \LL_1 (\x_i, \w^*, \fc)}{\smin ( \E{\nabla^2_w \LL_ (\x, \w^*, \fc)})}$
The empirical gradient is $\nabla \LL_m(\w^*, \fc)= \sum_{i=1}^m \frac{\nabla \LL_1 (\x_i, \w^*, \fc) }{m}$
where \allowdisplaybreaks{$
\nabla \mathcal{L}_1 (\x_i, \w^*, \fc) =  \begin{bmatrix} 
    \frac{f^c_1(x_i)}{\inner{\fc(\x_i)}{\w^*}} 
    \dots  
    \frac{f^c_l(x_i)}{\inner{\fc(\x_i)}{\w^*}} 
    \dots 
    \frac{ f^c_{k}(x_i) }{\inner{\fc(\x_i)}{\w^*}} 
    \end{bmatrix}_{(k)}
$.}
With the lower bound $\tau$ on $\inner{\fc}{\w^*}$, we can upper bound the gradient terms as, 
$$||\nabla \LL_1(\x, \w^*, \fc)||_2 \le  \frac{||\fc||_2}{\tau} \le  \frac{||\fc||_1}{\tau} \le \frac{1}{\tau}$$

As the gradient terms are decompositional and independent, using Hoeffding's inequality we have with probability at least $1-\frac{\delta}{2}$, 
\begin{equation} \label{eq:ineq2}
||\nabla \LL(\w^*, \fc) - \nabla \LL_m(\w^*, \fc)||_2  \le \frac{1}{2\tau}\sqrt{\frac{\log(\frac{4}{\delta})}{m}}     
\end{equation}

Let $\smin$ be the minimum eigen value of $\nabla^2\LL (\w^*, \fc)$. Using lemma~\ref{lemma:troop}, with probability atleast $1-\frac{\delta}{2}$, 
\begin{equation} \label{eq:troop}
\frac{\widehat \sigma_{\min}}{\smin} \ge 1- \tau \sqrt{\frac{\log(\frac{2k}{\delta})}{m}} 
\end{equation}

Pluging~\eqref{eq:ineq2} and~\eqref{eq:troop} in \eqref{eq:ineq1}, and taking union bound, we conclude that with probability atleast $1-\delta$, 
$$||\widehat \w_c - \w^* ||_2 \le \frac{1}{\kappa\tau} \Big(\smin- \smin\tau \sqrt{\frac{\log(\frac{2k}{\delta})}{m}}\Big)^{-1} (\sqrt{\frac{\log(\frac{4}{\delta})}{m}}) \le \frac{1}{\kappa \tau} \frac{1}{\smin} \Big(1 + \tau \sqrt{\frac{\log(\frac{2k}{\delta})}{m}}\Big) \sqrt{\frac{\log(\frac{4}{\delta})}{m}}$$
Neglecting the order m term and let $c = \frac{1}{\kappa\tau} $, we have,
$$||\widehat \w_c - \w^* ||_2 \le \frac{c}{\smin} \sqrt{\frac{\log(\frac{4}{\delta})}{m}}$$

\end{proof}

\begin{lemma} [Calibration Error with scaling] \label{lemma:platt} 
Assume a regular model $\G$ with injectivity, Lipschitz-continuity, twice differentiability, non-singular Hessian, and consistency is used to perform for re-calibration. With probability at least $1-\delta$, we have  
$$\CE{\widehat g}^2 - \CE{g^*}^2 \defeq   \comp(\frac{\log(\frac{2}{\delta})}{n})$$
\end{lemma}
\begin{proof}
Assume regularity conditions on the model class $\G_{\theta}$ (injectivity, Lipschitz-continuity, twice differentiability, non-singular Hessian, and consistency) as in Theorem 5.23 of \cite{stein1981estimation} hold true. Using injectivity property of the model class as in~\cite{kumar2019verified} we have for all $g_1, g_2\in \G$, 
\begin{equation} \label{eq:MSE}
\MSE{g_1} - \MSE{g_2} = \CE{g_1}^2 - \CE{g_2}^2    
\end{equation}
Let $\widehat g, g^* \in \G$ be models parameterized by $\widehat \theta$ and $\theta^*$ respectively. Using strong concavity of the empirical mean squared error we have,
$$\nMSE{\widehat g} \le \nMSE {g^*} + \inner{\nabla \nMSE{g^*}}{\widehat \theta - \theta^*} 
- \frac{\mu^2}{2} ||\widehat \theta - \theta^*||^2_2$$ 
where $\mu$ is the parameter constant for strong concavity. Re-arranging a few terms, we have,  
$$ \frac{\mu^2}{2} ||\widehat \theta - \theta^*||^2_2  \le \underbrace{\nMSE {g^*} - \nMSE{\widehat g}}_{\RN{1}} + \inner{\nabla \nMSE{g^*}}{\widehat \theta - \theta^*} $$ 
where term-$\RN{1}$ is less than zero because $\widehat \g$ is the empirical minimizer of the mean-squared error. Ignoring term-$\RN{1}$, we get: 
$$ \frac{\mu^2}{2} ||\widehat \theta - \theta^*||^2_2  \le  \inner{\nabla \nMSE{g^*}}{\widehat \theta - \theta^*} \le || \nabla \nMSE{g^*}||_2 ||{\widehat \theta - \theta^*}||_2 $$ 

As the assumed model class is Lipschitz wrt. $\theta$ the gradient bounded by Lipschitz constant $L = c_1$. $\E{\nabla \nMSE{g^*}} = 0$ as $g^*$ is the population minimizer. Using Hoeffding's bound for bounded function we have with probability at least $1-\delta$,
\begin{equation} \label{eq:HoeffMSE} 
||{\widehat \theta - \theta^*}||_2 \le \frac{c_1}{\mu^2} \sqrt{\frac{\log(\frac{2}{\delta})}{n}}
\end{equation}
Using the smoothness of the $\MSE{g}$, we have 
\begin{equation} \label{eq:smoothness}
\MSE{\widehat g} - \MSE{g^*} \le c_2 ||\widehat \theta - \theta^*||^2_2    
\end{equation}
where $c_2$ is the operator norm of the $\nabla^2\MSE{g^*} $. Combining~\eqref{eq:MSE},~\eqref{eq:HoeffMSE}, and~\eqref{eq:smoothness} we have for some universal constant $c = \frac{c_1c_2}{\mu^2}$ with probability at least $1-\delta$, 
\[
\CE{\widehat g}^2 - \CE{g^*}^2 \le   c \frac{\log(\frac{2}{\delta})}{n}
\]
\end{proof}

\begin{lemma} \label{lemma:err2}
Assume conditions from lemma \ref{lemma:err1} hold true. Additionally assume the learnt predictor $\fh$ is also bounded below at the non zero entries of $\w^*$ i.e. for all $\x$ such that $\pt(\x)>0$, we have $\sum_{y=1}^k \fh_y(\x) \w^*_y \ge \tau$ for some universal constant $\tau$. Let $\smin^{\fh}$ be the minimum eigenvalue of the Fisher information with predictor $\fh$. With probability at least $1-\delta$ we have 
\[
 || \wc - \widehat \w ||_2 \defeq \comp \left( \frac{1}{\sigma_{\min}^{\fh}}\left(\sqrt{\frac{\log(\frac{4}{\delta})}{m}} + ||\w^*||_2 \left( \sqrt{\frac{\log(\frac{4}{\delta})}{n}} + \min_{g \in \G} \CE{g} \right) \right) \right)
\]
\end{lemma}

\begin{proof}
Similar to lemma-\ref{lemma:err1}, 
% we have strong convexity on the empirical negative log-likelihood function which 
we represent with $\LL_m$ by absorbing the negative sign for simplified notation here on. Using the Taylor expansion we have, 
\[
\LL_m(\widehat \w, \widehat \f) \ge \LL_m(\wc, \widehat \f) + \inner{\nabla \LL_m(\wc, \widehat \f)}{\wh - \wc} + \frac{1}{2} (\wc - \widehat \w)^T \nabla^2\LL_m (\tilde\w, \fh)(\wc - \widehat \w)  
\]
% \[
% \LL_m(\wc, \fc) = \LL_m(\widehat \w, \fc) + \inner{\nabla \LL_m(\widehat \w, \fc)}{\wc - \widehat \w} + \frac{1}{2} (\wc - \widehat \w)^T \nabla^2\LL_m (\tilde\w, \fc)(\wc - \widehat \w) 
% \]
where $\tilde\w \in [\widehat\w, \wc] $. With the assumption $<\fh, \w^*> \ge \tau$, we have $\nabla^2\LL_m (\tilde\w, \fh) \ge \frac{\tau^2}{\min \ps(y)^2} \nabla^2\LL_m (\w^*, \fh)$ 
% \footnote{Instead we could have also used definition of self-concordance to get a lower bound with $\nabla^2\LL_m (\w^*, \fc)$.}
.  Let $\kappa = \frac{\tau^2}{\min \ps(y)^2}$. Using this we get,

$$ \LL_m(\wh, \fh) \ge \LL_m(\wc, \fh) + \inner{\nabla \LL_m(\wc, \fh)}{\wh - \wc} + \frac{\kappa}{2}(\wc - \widehat \w)^T \nabla^2\LL_m (\w^*, \fh)(\wc - \widehat \w)$$
$$ \underbrace{\LL_m(\wh, \fh) - \LL_m(\wc, \fh)}_{\RN{1}} \ge \inner{\nabla \LL_m(\wc, \fh)}{\wh - \wc} + \frac{\kappa}{2}(\wc - \widehat \w)^T \nabla^2\LL_m (\w^*, \fh)(\wc - \widehat \w)$$

where term-$\RN{1}$ is less than zero as $\wh$ is the minimizer of empirical NLL $\LL_m(\w, \fh)$. Ignoring that term and re-arranging a few terms we get, 
$$  -\inner{\nabla \LL_m(\wc, \fh)}{\wh - \wc} \ge \frac{\kappa}{2}(\wc - \widehat \w)^T \nabla^2\LL_m (\w^*, \fh)(\wc - \widehat \w)$$

With first order optimality on $\wc$, $\inner{\nabla \LL_m(\wc, \fc)}{\wh - \wc} \ge 0$. Using this we have: 
$$  \inner{\nabla \LL_m(\wc, \fc)}{\wh - \wc} -\inner{\nabla \LL_m(\wc, \fh)}{\wh - \wc} \ge \frac{\kappa}{2}(\wc - \widehat \w)^T \nabla^2\LL_m (\w^*, \fh)(\wc - \widehat \w)$$
$$  \inner{\nabla \LL_m(\wc, \fc)-\nabla \LL_m(\wc, \fh)}{\wh - \wc} \ge \frac{\kappa}{2}(\wc - \widehat \w)^T \nabla^2\LL_m (\w^*, \fh)(\wc - \widehat \w)$$

As before, let $\widehat \sigma_{\min}^{\fh}$ be the minimum eigenvalue of $\nabla^2\LL_m (\w^*, \fh)$. Using the fact that $(\wc - \w^*)^T \nabla^2\LL_m (\w^*, \fh)(\wc - \w^*) \ge \widehat \sigma_{\min}^{\fh} ||\wc - \w^* ||_2^2$, we get,
$$  \inner{\nabla \LL_m(\wc, \fc)-\nabla \LL_m(\wc, \fh)}{\wh - \wc} \ge \frac{\kappa \widehat \sigma_{\min}^{\fh}}{2}||\wc - \widehat \w||_2^2$$

Using Holder's inequality on LHS and slight re-arranging gives, 
\begin{equation} \label{eq:ineq3}
||\nabla \LL_m(\wc, \fc)-\nabla \LL_m(\wc, \fh)||_2 \ge \frac{\kappa \widehat \sigma_{\min}^{\fh} }{2} ||\wc -\wh ||_2 
\end{equation}

From lemma~\ref{lemma:err1}, we have $\wc$ converging in probability to $\w^*$. Thus by definition of convergence, lower bound assumptions $\sum_{y=1}^k \fh_y(\x) \w^*_y \ge \tau$ and $\sum_{y=1}^k \fc_y(\x) \w^*_y \ge \tau$ implies for large enough $m$ we have, $\sum_{y=1}^k \fh_y(\x) \wc_y \ge \tau$ and $\sum_{y=1}^k \fc_y(\x) \wc_y \ge \tau$. With this, we have:  
% Lipschitzness on the gradient $\nabla\LL_m(\wc, \f) $ with respect to $\f$ with Lipschitz constant $l$, 
% $$ $$
$$|| \nabla \LL_m(\wc, \widehat \f) - \nabla \LL_m( \wc, \fc)||_2 \le \sum_{i=1}^m \frac{1}{m} || \nabla \LL_1(\x_i, \wc, \widehat \f) - \nabla \LL_1( \x_i, \wc, \fc)||_2 \le \frac{1}{\tau^2} \sum_{i=1}^m \frac{1}{m} || \widehat \f(\x_i) - \fc(\x_i) ||_2$$

Adding and subtracting $\E{\sum_{i=1}^m \frac{1}{m} || \widehat \f(\x_i) - \fc(\x_i) ||_2}$ in RHS, we get, 
\begin{equation}
\begin{split}
|| \nabla \LL_m(\wc, \widehat \f) - \nabla \LL_m( \wc, \fc)||_2  \le \frac{1}{\tau^2} \Big( & \underbrace{\sum_{i=1}^m \frac{1}{m} || \widehat \f(\x_i) - \fc(\x_i) ||_2  - \E{\sum_{i=1}^m \frac{1}{m} || \widehat \f(\x_i) - \fc(\x_i) ||_2}}_{\RN{1}}  \\& \qquad +  \underbrace{\E{\sum_{i=1}^m \frac{1}{m} || \widehat \f(\x_i) - \fc(\x_i) ||_2}}_{\RN{2}} \Big) 
\end{split} \label{eq:bound_grad}
\end{equation}
% \begin{equation} \label{eq:gradlip}   
% \end{equation}

We bound the term-$\RN{1}$ using Hoeffdings inequality and term-$\RN{2}$ using calibration error. For term-1, using Hoeffdings inequality for the bounded function,  we have with probability $1-\frac{\delta}{2}$, 
\begin{equation} \label{eq:term1_bound}
\sum_{i=1}^m \frac{1}{m} || \widehat \f(\x_i) - \fc(\x_i) ||_2  - \E{\sum_{i=1}^m \frac{1}{m} || \widehat \f(\x_i) - \fc(\x_i) ||_2} \le \sqrt{\frac{\log(\frac{4}{\delta})}{m}}     
\end{equation}

Consider term-$\RN{2}$, 
\begin{align*}
  \E{\sum_{i=1}^m \frac{1}{m} || \widehat \f(\x_i) - \fc(\x_i) ||_2} &= \mathbb{E}_{\x \sim \T}\left[|| \widehat \f (\x) - \fc (\x) ||_2\right]  \\
  &= \mathbb{E}_{\x \sim \Ss}\left[ \frac{\pt(\x)}{\ps(\x)} || \widehat \f (\x) - \fc(\x) ||_2\right] \\ 
  &\le \mathbb{E}_{\x \sim \Ss}\left[ \max_y \frac{\pt(y)}{\ps(y)} || \widehat \f (\x) - \fc(\x) ||_2\right] \\
  &\le \max_y \frac{\pt(y)}{\ps(y)} \mathbb{E}_{\x \sim \Ss}\left[ || \widehat \f (\x) - \fc(\x) ||_2\right] \numberthis \label{eq:term2_bound}
\end{align*}

Using Jensen's inequality on RHS, we get $$\mathbb{E}_{\x \sim \Ss}{|| \widehat \f - \fc ||_2} \le \left(\mathbb{E}_{\x \sim \Ss}{|| \widehat \f - \fc ||^2_2}\right)^{\frac{1}{2}} = \CE{\fh}$$ 

Depending on the degree of the miscalibration and method involved to calibrate we can bound the $\CE{\widehat \f}$. For example, if using vector scaling on a held out training data for calibration, we can use lemma-\ref{lemma:platt} to bound the calibration error $\CE{\widehat \f}$ i.e. with probability at least $1-\frac{\delta}{2}$, we have, 
\begin{equation} \label{eq:calib_err}
\CE{\fh} \le \sqrt{\CE{\f^*}^2 + c \frac{\log(\frac{4}{\delta})}{n}} \le  \min_{\g \in \G} \CE{\g \circ \fh } + \sqrt{c\frac{\log(\frac{4}{\delta})}{n}}    
\end{equation}
 
 Let $\sigma_{\min}^{\fh}$ be the minimum eigen value of $\nabla^2\LL (\w^*, \fh)$. Using lemma~\ref{lemma:troop}, with probability atleast $1-\frac{\delta}{2}$, 
\begin{equation} \label{eq:troop2}
\frac{\widehat \sigma_{\min}^{\fh}}{\sigma_{\min}^{\fh}} \ge 1- \tau \sqrt{\frac{\log(\frac{2k}{\delta})}{m}} 
\end{equation}

% In equation, 
% ~\eqref{eq:gradlip}
% one na\"ive bound on $l(\wc)$ is $\comp(\frac{1}{\tau^2})$. 
Combining equations \eqref{eq:troop2}, \eqref{eq:term1_bound}, \eqref{eq:term2_bound}, \eqref{eq:calib_err}, \eqref{eq:bound_grad}
% $~\eqref{eq:gradlip}$ 
into equation  \eqref{eq:ineq3}
% ~\eqref{eq:caliberr}
, we have with probability atleast $1-\delta$,  
\begin{align*}
    || \wc - \widehat \w ||_2 &\le \frac{1}{\kappa \sigma_{\min}^{\fh} \tau^2}\left(\sqrt{\frac{\log(\frac{4}{\delta})}{m}} + \max_y \frac{\pt(y)}{\ps(y)} \left( \sqrt{c \frac{\log(\frac{4}{\delta})}{n}} + \min_{g \in \G} \CE{g} \right) \right) \Big(1- \tau \sqrt{\frac{\log(\frac{2k}{\delta})}{m}}\Big)^{-1} \\
   &\le \frac{1}{\kappa \sigma_{\min}^{\fh} \tau^2}\left(\sqrt{\frac{\log(\frac{4}{\delta})}{m}} + ||\w^*||_2 \left( \sqrt{c\frac{\log(\frac{4}{\delta})}{n}} + \min_{g \in \G} \CE{g} \right) \right) \Big(1+ \tau \sqrt{\frac{\log(\frac{2k}{\delta})}{m}}\Big)
\end{align*}

Neglecting the order $m$ and $\sqrt{mn}$ terms, we get with probability at least $1-\delta$, 
$$ || \wc - \widehat \w ||_2 \le \frac{1}{\kappa \sigma_{\min}^{\fh} \tau^2}\left(\sqrt{\frac{\log(\frac{4}{\delta})}{m}} + ||\w^*||_2 \left( \sqrt{c\frac{\log(\frac{4}{\delta})}{n}} + \min_{\g \in \G} \CE{
\g \circ \fh } \right) \right)  $$

\end{proof}

\begin{lemma} \label{lemma:support}
Assume $||\widehat \theta||_1 = ||\theta||_1 = 1$. Let's consider a non-zero support of $\theta$ be denotes by a set s, then if $||\theta^s
- \widehat \theta^s||_2 \le \epsilon$ implies $||\theta- \widehat \theta||_2 \le 2\epsilon$.  
\end{lemma}
\begin{proof}
Assume $z$ is the subset of entries for which $\tp$ is zero. Given $||\tz^s- \tp^s||_2 \le \epsilon$. We want to bound $||\tp^z - \tz^z||_2 = ||\tz^z||_2$.  We can re-write $||\tz^z||^2_1 = || 1- \tz^s||^2_1 = || \tp^s - \tz^s||^2_1 = (\sum_{i\in s} \tp^s_i - \tz^s_i)^2$. Assume $a_i = \tp^s_i - \tz^s_i$, we have
\begin{align*}
(\sum_{i\in z} a_i)^2 &= (\sum_{i \in s} a_i)^2 = \sum_{i\in s} a_i^2 + 2 \sum_{\substack{i,j\in s \\ i\ne j}} a_i a_j \\
&= \sum_{i\in s} a_i^2 + 2 \sum_{\substack{i\in s \\ j \in z}} a_i (-a_i - a_j) \\ 
&= \sum_{i\in s} a_i^2 + 2 \sum_{i\in s} -a_i^2 - 2\sum_{\substack{i\in s\\j\in z}} a_ia_j \\
&= -\sum_{i\in s} a_i^2  - 2\sum_{j\in z} a_j \sum _{i\in s}a_i  \\
&= -\sum_{i\in s} a_i^2  + 2(\sum_{i\in z} a_j)^2  \\
\end{align*}
Thus we have $(\sum_{i\in z} a_i)^2 = \sum_{i\in s} a_i^2$. Using the fact that $l1$-norm is greater than $l2$-norm, $\sum_{i\in z} a_i^2 \le \sum_{i\in s} a_i^2 \le \epsilon$. Hence $||\tp- \tz ||_2 \le 2\epsilon$.     
\end{proof}

\section{Connection of IPM methods} \label{apx:IPM}
% Maybe we can shift this to appendix. 
\begin{lemma}
Consider a kernel with feature vector $\phi(\widehat y) = e_{\widehat y} \in \mathbb{R}^{|\mathcal{Y}|}$ such that $e_x$ is one at $x^{th}$ position and zero everywhere else. With this RKHS kernel the obtained MMD formulation is equivalent to CO2 defined above.
\end{lemma}
\begin{proof}
\begin{align*}
\mu^{\widehat y}_q &= E_{ y \sim q(\widehat y)} (\phi (y)) = q(\widehat y) \\
\mu^{\widehat y}_{q'} &= E_{ y \sim q'(\widehat y)} (\phi (y))
= q'(\widehat y) \\  
&\quad = \sum_y p(\widehat y| y) w(y) p(y) = Cw 
\end{align*}
Hence $\argmin_w MMD^2 = \argmin_w ||\mu^{\widehat y}_q - \mu^{\widehat y}_{q'} ||_2^2 = \argmin_w || q - Cw||^2_2 $ 
\end{proof}
